# Supplementary material for: Hierarchical Block Structures and High-resolution Model Selection in Large Networks
Source: arXiv:1310.4377 source file (2014-03-25)
Supplement: Supplementary file 1 [file sup_inf.pdf]

# Supplemental Material: Hierarchical block structures and high-resolution model selection in large networks

Tiago P. Peixoto\*

*Institut für Theoretische Physik, Universität Bremen, Hochschulring 18, D-28359 Bremen, Germany*

## A. Empirical networks

In Fig. 1 is shown a higher resolution version of Fig. 6 in the main text, with additional information on the correlation with geographical location. As can be seen, at the topmost level it is separated into four blocks, comprising: 1. The “core” AS nodes; 2. The Americas, Australia and

East Asia; 3. Europe, Africa, South Asia and the Middle East; 4. Russia and Western Europe. These get further subdivided in the lower levels.

In Fig. 2 is shown a higher resolution version of Fig. 7 in the main text, containing the large-scale structure of the IMDB network. See also Ref. [1] for more details on the type of information which can be associated with each block.

- 
- [1] T. P. Peixoto, Physical Review Letters **110**, 148701 (2013).

---

\* tiago@itp.uni-bremen.de

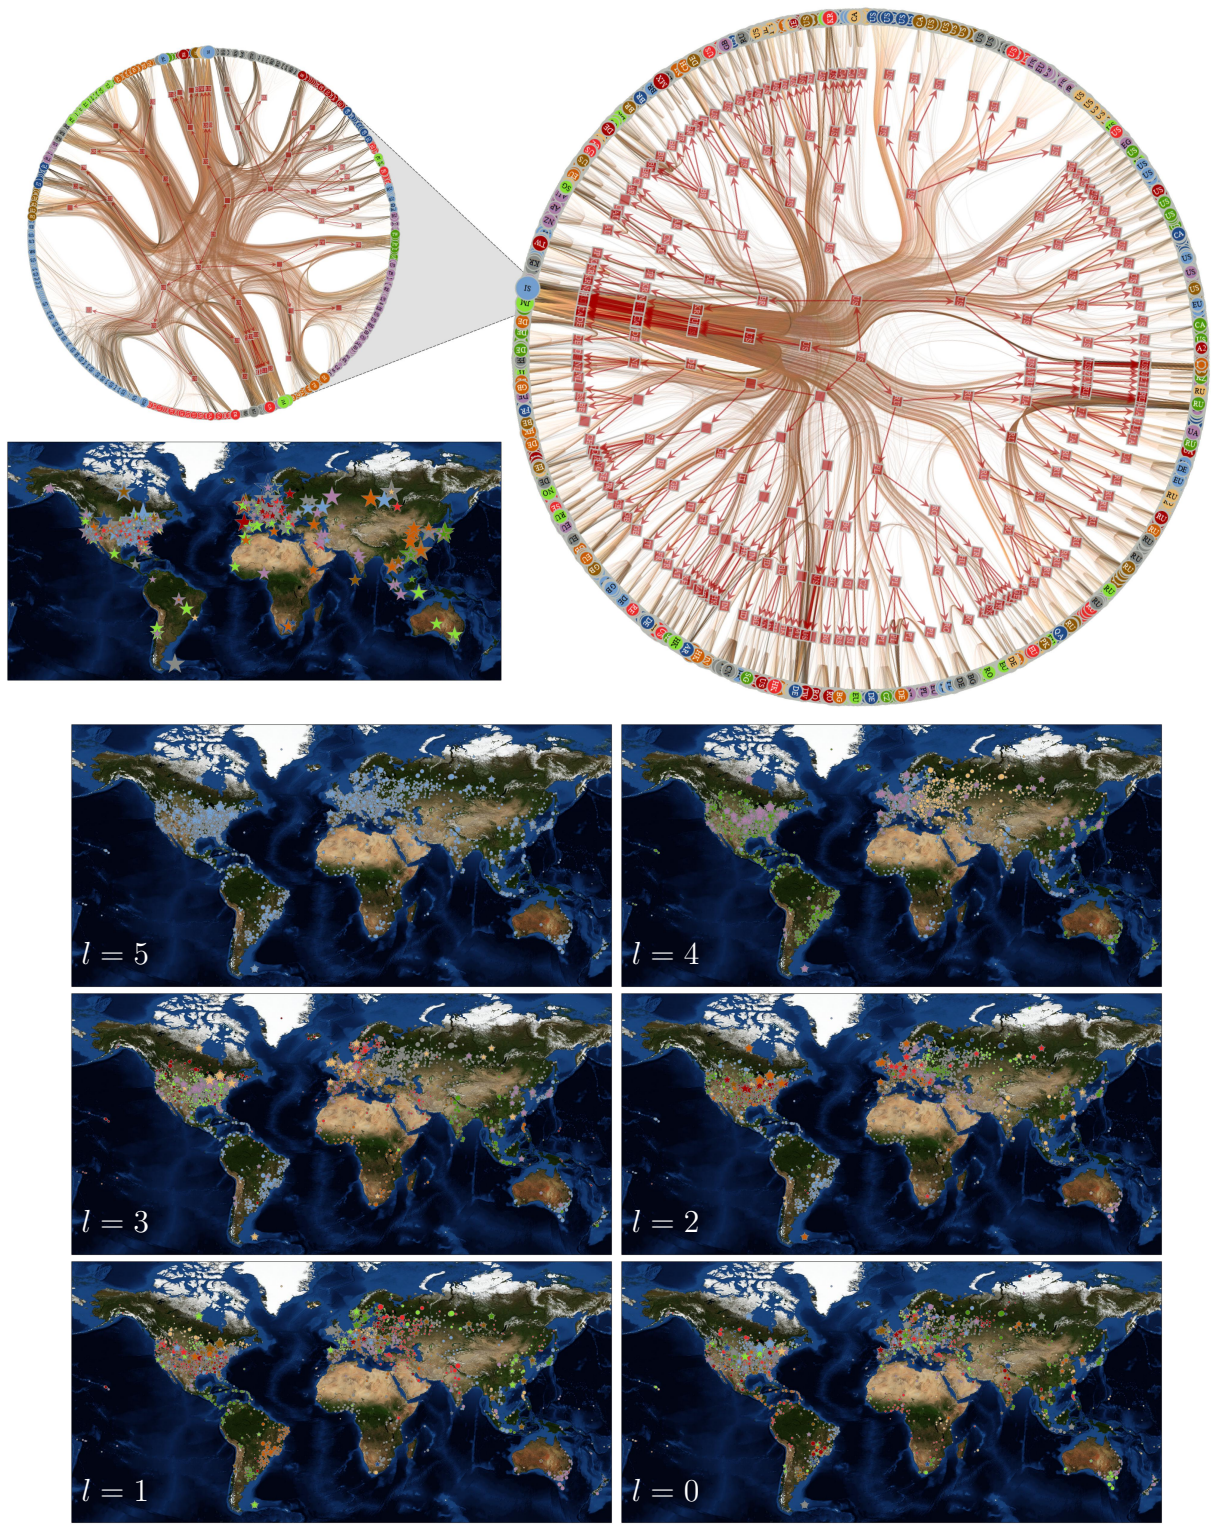

FIG. 1. Large-scale structure of the Internet at the autonomous systems level, as obtained by the nested stochastic block model, displaying a prominent core-periphery architecture. The “blow up” shows the nodes which belong to the “core” top-level branch, containing AS nodes spread all over the globe, as shown in the map inset below it. The maps at the bottom show the network partitions at different hierarchical levels, from top to bottom, showing the strong correlation with geographical divisions. The stars ( $\star$ ) are the “core” nodes, and the circles are regular AS nodes.

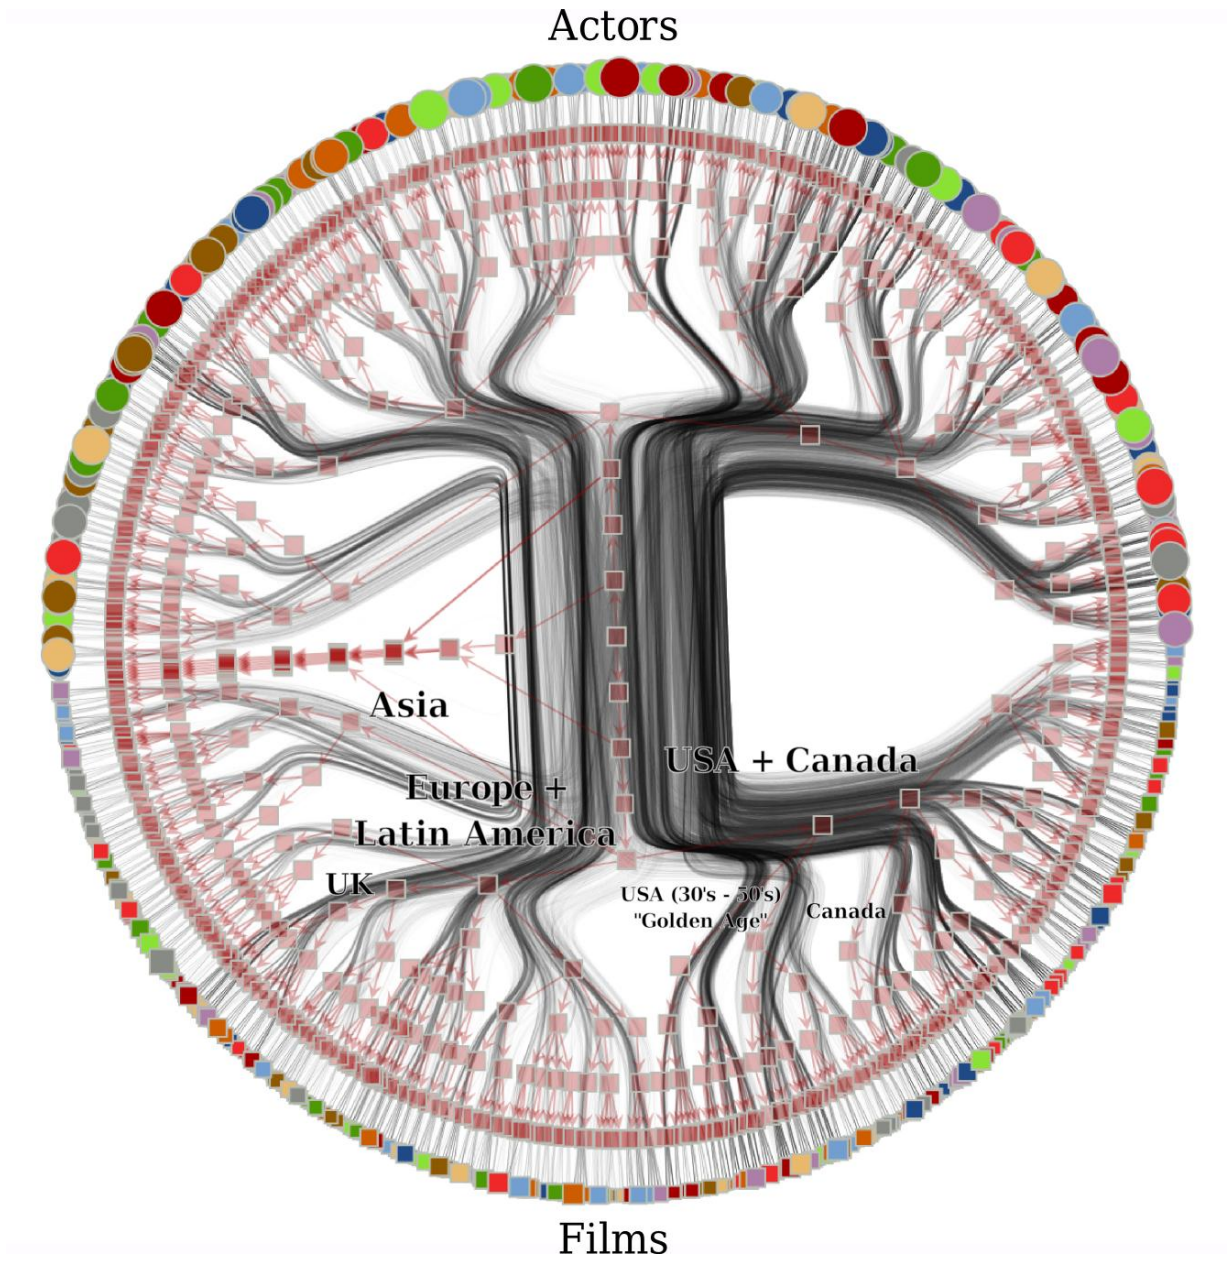

FIG. 2. Large-scale structure of the IMDB actor-film network. Each node in this graph represents a lowest-level block in the hierarchy, instead of individual nodes in the graph. The size of the nodes indicates the number of nodes in each group. The hierarchy branch at the top are the actors, and at the bottom are the films. The labels classify each branch according to the most prominent geographical, temporal or genre characteristics found in the database.
